# Supplementary material for: Deformable Filter Convolution for Point Cloud Reasoning
Source: arXiv:1907.13079 source file (2019-07-30)
Supplement: Supplementary file 1 [file fig_filter_supp.tex]

% !TEX root = ../supp.tex
\begin{figure*}[h!]
\centering
\begin{minipage}{\textwidth}
\centering
\begin{tabular}{c c c}
\multirow{2}{*}{PCC}             & 
\includegraphics[width=0.45\textwidth,trim={0 0.8cm 0 0.8cm},clip]{figures/kernel_supp/contconv_filter_supp/contconv_filter_layer1_1_car} & 
\includegraphics[width=0.45\textwidth,trim={0 0.8cm 0 0.8cm},clip]{figures/kernel_supp/contconv_filter_supp/contconv_filter_layer2_1_car} \\
                                 & 
\includegraphics[width=0.45\textwidth,trim={0 0.8cm 0 0.8cm},clip]{figures/kernel_supp/contconv_filter_supp/contconv_filter_layer1_2_car} & 
\includegraphics[width=0.45\textwidth,trim={0 0.8cm 0 0.8cm},clip]{figures/kernel_supp/contconv_filter_supp/contconv_filter_layer2_2_car} \\
                                 & {\footnotesize Layer 1}                                                        
                                 & {\footnotesize Layer 2}                                           \\
                                 \\
\multirow{2}{*}{Ours}            & 
\includegraphics[width=0.45\textwidth,trim={0 0.8cm 0 0.8cm},clip]{figures/kernel_supp/cont_filter_supp/cont_filter_layer1_1_car}     & 
\includegraphics[width=0.45\textwidth,trim={0 0.8cm 0 0.8cm},clip]{figures/kernel_supp/cont_filter_supp/cont_filter_layer2_1_car}     \\
                                 & 
\includegraphics[width=0.45\textwidth,trim={0 0.8cm 0 0.8cm},clip]{figures/kernel_supp/cont_filter_supp/cont_filter_layer1_2_car}     & 
\includegraphics[width=0.45\textwidth,trim={0 0.8cm 0 0.8cm},clip]{figures/kernel_supp/cont_filter_supp/cont_filter_layer2_2_car}     \\
                                 & {\footnotesize Layer 1}                                                        
                                 & {\footnotesize Layer 2}                                           \\
\end{tabular}
\end{minipage}
\vspace{0.05in}
\caption{Visualization of our learned 3D filters ($3 \times 3 \times 3$) trained on KITTI car
detection.}
\label{fig:filtervizsupp1}
\end{figure*}

\begin{figure*}[h]
\centering
\begin{minipage}{\textwidth}
\centering
\begin{tabular}{c c c}
\multirow{2}{*}{PCC}             & 
\includegraphics[width=0.45\textwidth,trim={0 0.8cm 0 0.8cm},clip]{figures/kernel_supp/contconv_filter_supp/contconv_filter_layer1_1_ped} & 
\includegraphics[width=0.45\textwidth,trim={0 0.8cm 0 0.8cm},clip]{figures/kernel_supp/contconv_filter_supp/contconv_filter_layer2_1_ped} \\
                                 & 
\includegraphics[width=0.45\textwidth,trim={0 0.8cm 0 0.8cm},clip]{figures/kernel_supp/contconv_filter_supp/contconv_filter_layer1_2_ped} & 
\includegraphics[width=0.45\textwidth,trim={0 0.8cm 0 0.8cm},clip]{figures/kernel_supp/contconv_filter_supp/contconv_filter_layer2_2_ped} \\
                                 & {\footnotesize Layer 1}                                                        
                                 & {\footnotesize Layer 2}                                           \\
                                 \\
\multirow{2}{*}{Ours}            & 
\includegraphics[width=0.45\textwidth,trim={0 0.8cm 0 0.8cm},clip]{figures/kernel_supp/cont_filter_supp/cont_filter_layer1_1_ped}     & 
\includegraphics[width=0.45\textwidth,trim={0 0.8cm 0 0.8cm},clip]{figures/kernel_supp/cont_filter_supp/cont_filter_layer2_1_ped}     \\
                                 & 
\includegraphics[width=0.45\textwidth,trim={0 0.8cm 0 0.8cm},clip]{figures/kernel_supp/cont_filter_supp/cont_filter_layer1_2_ped}     & 
\includegraphics[width=0.45\textwidth,trim={0 0.8cm 0 0.8cm},clip]{figures/kernel_supp/cont_filter_supp/cont_filter_layer2_2_ped}     \\
                                 & {\footnotesize Layer 1}                                                        
                                 & {\footnotesize Layer 2}                                           \\
\end{tabular}
\end{minipage}
\vspace{0.05in}
\caption{Visualization of our learned 3D filters ($3 \times 3 \times 3$) trained on KITTI pedestrian
detection.}
\label{fig:filtervizsupp2}
\vspace{-0.1in}
\end{figure*}
